# Supplementary material for: OEDIPUS: An Experiment Design Framework for Sparsity-Constrained MRI
Source: arXiv:1805.00524 source file (2019-01-04)
Supplement: Supplementary file 1 [file OEDIPUS_supplementary.pdf]

# Supplementary Material for “OEDIPUS: An Experiment Design Framework for Sparsity-Constrained MRI”

Justin P. Haldar, *Senior Member, IEEE,* and Daeun Kim, *Student Member, IEEE*

TABLE SI
TABLE OF NRMSE VALUES FOR RECONSTRUCTED SINGLE-CHANNEL 2D T2-WEIGHTED BRAIN DATA. RESULTS ARE SHOWN FOR WAVELET (WAV) AND TOTAL VARIATION (TV) RECONSTRUCTION APPROACHES, AND FOR UNIFORM (UNI), RANDOM (RAND), AND OEDIPUS SAMPLING PATTERNS.

| | | **Third Subject** | | | | **Fourth Subject** | | | | **Fifth Subject** | | | | **Sixth Subject** | | | | **Seventh Subject** | | | |
|---|---|---|---|---|---|---|---|---|---|---|---|---|---|---|---|---|---|---|---|---|---|
| | | **Uni** | **Rand** | **SCO** | **MCO** | **Uni** | **Rand** | **SCO** | **MCO** | **Uni** | **Rand** | **SCO** | **MCO** | **Uni** | **Rand** | **SCO** | **MCO** | **Uni** | **Rand** | **SCO** | **MCO** |
| $R = 2$ | **Wav** | 0.873 | 0.154 | **0.120** | 0.337 | 0 865 | 0.181 | **0.129** | 0.316 | 0.882 | 0.157 | **0.127** | 0.344 | 0.853 | 0.203 | **0.147** | 0.337 | 0.859 | 0.181 | **0.131** | 0.327 |
| | **TV** | 0.789 | 0.119 | **0.101** | 0.195 | 0.829 | 0.150 | **0.108** | 0.424 | 0.808 | 0.128 | **0.103** | 0.241 | 0.832 | 0.168 | **0.112** | 0.404 | 0.886 | 0.141 | **0.105** | 0.189 |

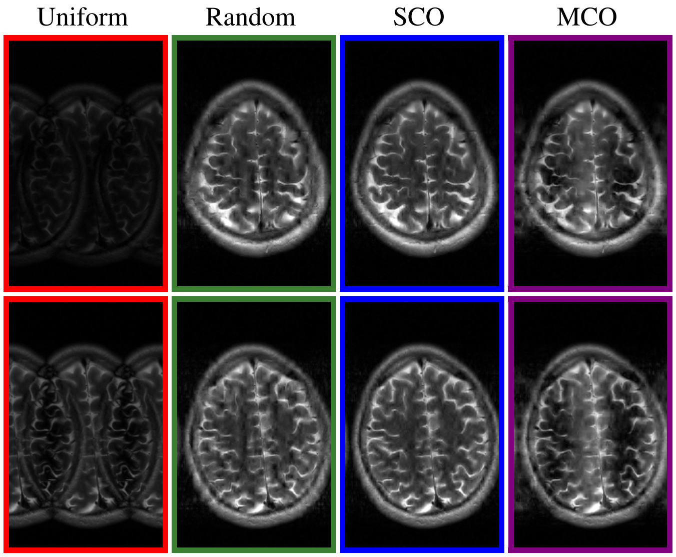


Fig. S1. Reconstruction results for wavelet-regularized single-channel 2D T2-weighted brain data with $R = 2$. The top row shows results from the first subject, while the bottom row shows results from the second.

TABLE SII
TABLE OF NRMSE VALUES FOR RECONSTRUCTED MULTI-CHANNEL 2D T2-WEIGHTED BRAIN DATA. RESULTS ARE SHOWN FOR WAVELET (WAV) AND TOTAL VARIATION (TV) RECONSTRUCTION APPROACHES, AND FOR UNIFORM (UNI), RANDOM (RAND), AND OEDIPUS SAMPLING PATTERNS.

| | | **Third Subject** | | | | **Fourth Subject** | | | | **Fifth Subject** | | | | **Sixth Subject** | | | | **Seventh Subject** | | | |
|---|---|---|---|---|---|---|---|---|---|---|---|---|---|---|---|---|---|---|---|---|---|
| | | **Uni** | **Rand** | **SCO** | **MCO** | **Uni** | **Rand** | **SCO** | **MCO** | **Uni** | **Rand** | **SCO** | **MCO** | **Uni** | **Rand** | **SCO** | **MCO** | **Uni** | **Rand** | **SCO** | **MCO** |
| $R = 2$ | **Wav** | **0.048** | 0.051 | 0.057 | 0.050 | **0.055** | 0.059 | 0.063 | 0.057 | **0.048** | 0.053 | 0.059 | 0.052 | **0.050** | 0.057 | 0.062 | 0.054 | **0.051** | 0.055 | 0.059 | 0.052 |
| | **TV** | **0.047** | 0.048 | 0.054 | 0.049 | **0.054** | 0.055 | 0.059 | 0.055 | **0.046** | 0.050 | 0.056 | 0.050 | **0.047** | 0.052 | 0.057 | 0.050 | **0.048** | **0.048** | 0.053 | **0.048** |
| $R = 3$ | **Wav** | 0.079 | 0.086 | 0.085 | **0.072** | 0.092 | 0.098 | 0.092 | **0.080** | 0.089 | 0.92 | 0.090 | **0.075** | 0.098 | 0.103 | 0.095 | **0.080** | 0.093 | 0.098 | 0.892 | **0.077** |
| | **TV** | 0.068 | 0.076 | 0.079 | **0.067** | 0.078 | 0.085 | 0.086 | **0.074** | 0.072 | 0.082 | 0.084 | **0.069** | 0.080 | 0.089 | 0.086 | **0.071** | 0.076 | 0.081 | 0.082 | **0.069** |
| $R = 4$ | **Wav** | 0.124 | 0.140 | 0.106 | **0.093** | 0.148 | 0.150 | 0.111 | **0.101** | 0.157 | 0.140 | 0.111 | **0.098** | 0.195 | 0.167 | 0.119 | **0.109** | 0.187 | 0.158 | 0.112 | **0.102** |
| | **TV** | 0.107 | 0.117 | 0.100 | **0.085** | 0.129 | 0.125 | 0.106 | **0.091** | 0.119 | 0.127 | 0.119 | **0.089** | 0.137 | 0.142 | 0.113 | **0.093** | 0.134 | 0.132 | 0.105 | **0.088** |

J. Haldar and D. Kim are with the Signal and Image Processing Institute, Ming Hsieh Department of Electrical Engineering, University of Southern California, Los Angeles, CA, 90089, USA.

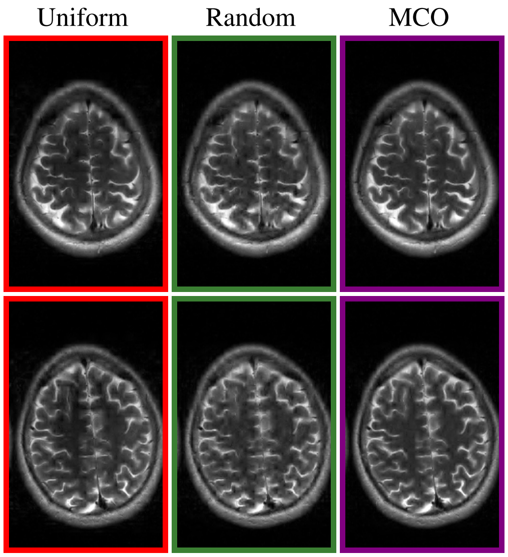


Fig. S2. Reconstruction results for wavelet-regularized multi-channel 2D T2-weighted brain data with $R = 4$. The top row shows results from the first subject, while the bottom row shows results from the second.

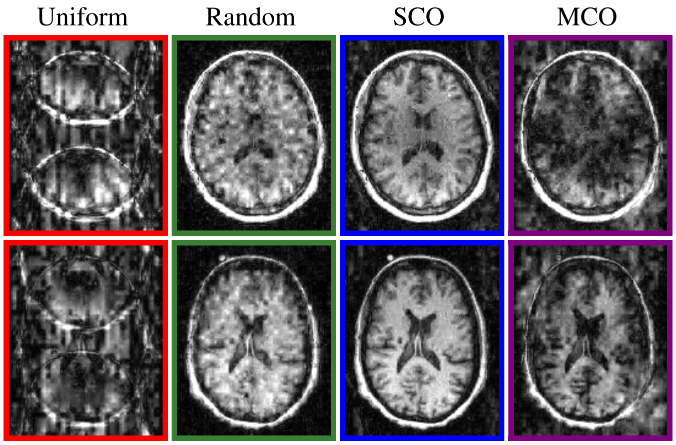


Fig. S3. Reconstruction results for wavelet-regularized single-channel 3D T1-weighted brain data with $R = 4$. The top row shows results from the healthy subject, while the bottom row shows results from the stroke subject.

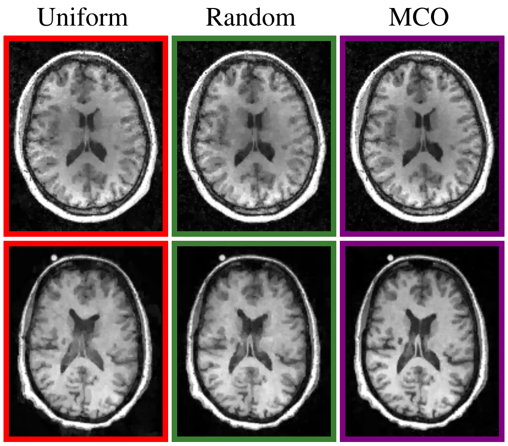


Fig. S4. Reconstruction results for TV-regularized multi-channel 3D T1-weighted brain data with $R = 8$. The top row shows results from the healthy subject, while the bottom row shows results from the stroke subject.

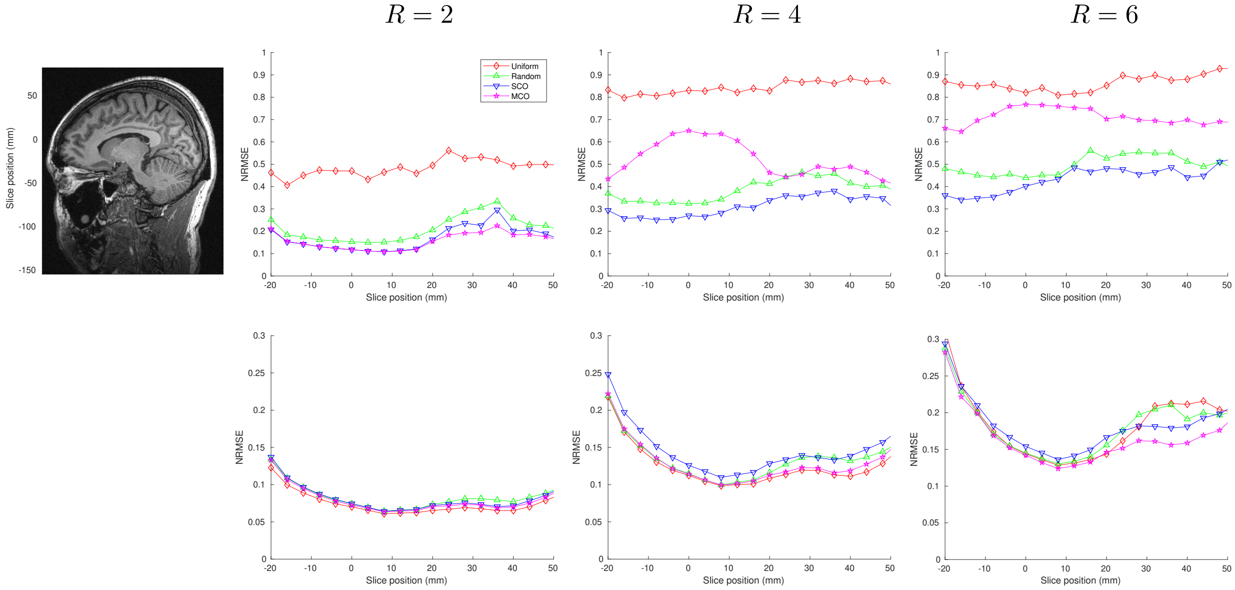


Fig. S5. Volumetric reconstruction results for wavelet-regularized 3D T1-weighted brain data from the healthy subject. Results are shown for both (top) single-channel and (bottom) multi-channel cases. The plots show NRMSE as a function of spatial position for different acceleration factors. We also show a sagittal reference image, where the origin of the spatial coordinate system is defined as the location of the single-slice shown in Fig. 3 from the main manuscript.

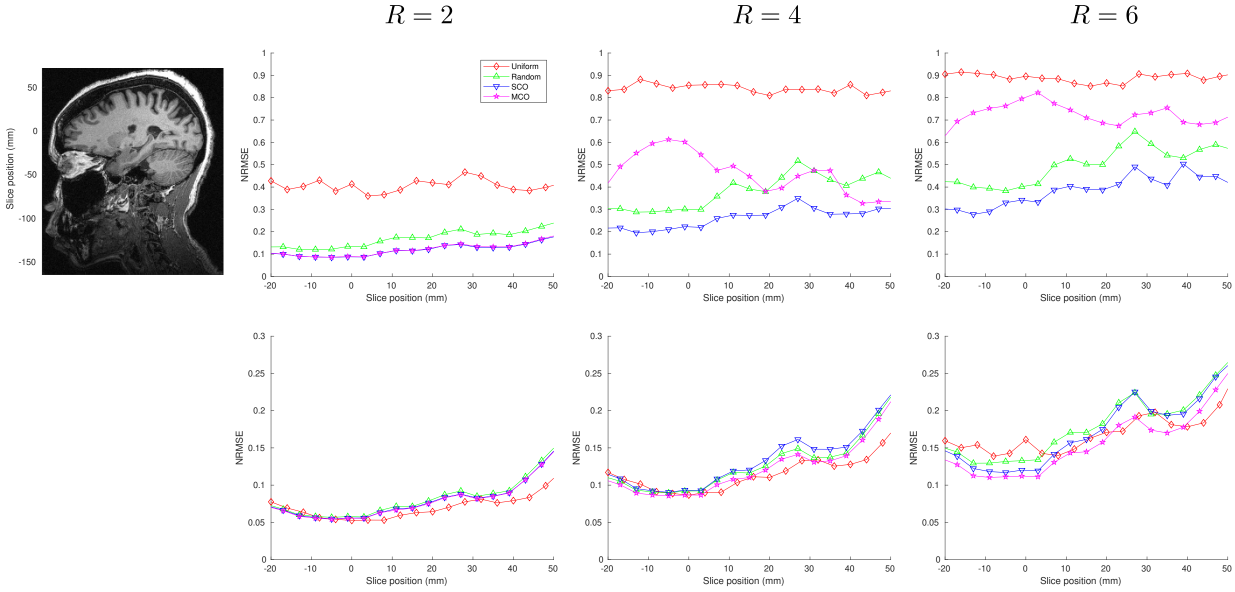


Fig. S6. Volumetric reconstruction results for wavelet-regularized 3D T1-weighted brain data from the stroke subject. Results are shown for both (top) single-channel and (bottom) multi-channel cases. The plots show NRMSE as a function of spatial position for different acceleration factors. We also show a sagittal reference image, where the origin of the spatial coordinate system is defined as the location of the single-slice shown in Fig. 3 from the main manuscript.
